# Supplementary material for: Exceptional points as signatures of dynamical magnetic phase transitions
Source: arXiv:2205.02308 ancillary file (2023-03-06)
Supplement: Supplementary file 1 [file Supplementary_Material.pdf]

# Supplementary Material for "Exceptional points as signatures of dynamical magnetic phase transitions"

Kuangyin Deng,* Xin Li, and Benedetta Flebus†
*Department of Physics, Boston College, 140 Commonwealth Avenue, Chestnut Hill, Massachusetts 02467, USA*

In this supplemental material, we provide a detailed derivation of the non-Hermitian Hamiltonian associated with the dynamics of Eqs. (2) and (3) of the main text.

## I. EFFECTIVE NON-HERMITIAN HAMILTONIAN

Assuming the magnetic field to lie in the $xz$ plane, i.e., $\mathbf{B} = B(\cos\Theta,\, 0,\, \sin\Theta)$, the classical energy corresponding to Eq. (1) of the main text can be written as

$$\begin{aligned} E^{cl}_{total} =& \gamma B_0 S(\cos\Theta\cos\phi_A\cos\theta_A + \sin\Theta\sin\theta_A + \cos\Theta\cos\phi_B\cos\theta_B + \sin\Theta\sin\theta_B) \\ &+ KS^2(\sin^2\theta_A + \sin^2\theta_B) + JS^2(\cos\phi_{AB}\cos\theta_A\cos\theta_B + \sin\theta_A\sin\theta_B). \end{aligned} \tag{S.1}$$

where $\phi_{A(B)}$ and $\theta_{A(B)}$ are, respectively, the azimuthal and cant angle of the macrospin $\mathbf{S}_{A(B)}$, while $\phi_{AB} = \phi_A - \phi_B$. Minimization of Eq. (S.1) with respect to $\theta_{A(B)}, \phi_{A(B)}$ gives the ground-state spin configuration.

For the macrospin $\mathbf{S}_{A(B)}$, we can orient a spin-space Cartesian coordinate system such that the new $\hat{z}$ axis locally lies along the classical orientation of $\tilde{\mathbf{S}}_{A(B)}$. The latter can be related to the classical orientation of the macrospin $\mathbf{S}_{A(B)}$ in the global frame of reference via the transformation

$$\mathbf{S}_i = \mathcal{R}^i_{LG}\tilde{\mathbf{S}}_i\,. \tag{S.2}$$

Here we have introduced $\mathcal{R}^i_{LG} = \mathcal{R}_z(\phi_i)\mathcal{R}_y(\theta_i)$, where

$$\mathcal{R}_y(\theta_i) = \begin{pmatrix} \sin\theta_i & 0 & \cos\theta_i \\ 0 & 1 & 0 \\ -\cos\theta_i & 0 & \sin\theta_i \end{pmatrix} \qquad \mathcal{R}_z(\phi_i) = \begin{pmatrix} \cos\phi_i & -\sin\phi_i & 0 \\ \sin\phi_i & \cos\phi_i & 0 \\ 0 & 0 & 1 \end{pmatrix} \tag{S.3}$$

describes a right-handed rotation by an angle $\phi_i(\theta_i)$ about the global $\hat{z}(\hat{y})$ axis, and $i = A, B$. Far below the magnetic ordering temperature, we can access the magnon spectrum by linearizing the Holstein-Primakoff transformation in the local frame of reference, i.e.

$$\tilde{S}^+ = \tilde{S}^x + i\tilde{S}^y = \sqrt{2S}\sqrt{1 - \frac{d_i^\dagger d_i}{2S}}\, d_i \approx \sqrt{2S}d_i\,, \qquad \tilde{S}^z = S - d_i^\dagger d_i\,, \tag{S.4}$$

where $d_i(d_i^\dagger)$ is the magnon annihilation (creation) operator of the layer $i$, obeying the bosonic commutation relation $[d_i, d_j^\dagger] = \delta_{ij}$. Equations (2) and (3) of the main text can be rewritten as

$$(1+\alpha_A^2)\frac{\mathrm{d}\mathbf{S}_A}{\mathrm{d}t} = -\gamma\mathbf{S}_A\times\mathbf{B}^{\text{eff}}_A - \frac{\gamma\alpha_A}{S}\mathbf{S}_A\times(\mathbf{S}_A\times\mathbf{B}^{\text{eff}}_A), \tag{S.5}$$

$$(1+\alpha_B^2)\frac{\mathrm{d}\mathbf{S}_B}{\mathrm{d}t} = -\gamma\mathbf{S}_B\times\mathbf{B}^{\text{eff}}_B - \frac{\gamma\alpha_B}{S}\mathbf{S}_B\times(\mathbf{S}_B\times\mathbf{B}^{\text{eff}}_B)\,. \tag{S.6}$$

* dengku@bc.edu
† flebus@bc.edu

In local coordinates, Eqs. (S.5) and (S.6) become

$$\begin{aligned}
(1+\alpha_A^2)\frac{\mathrm{d}\tilde{\mathbf{S}}_A}{\mathrm{d}t} =&\tilde{\mathbf{S}}_A \times \Big[-\gamma\tilde{\mathbf{B}}_A - J(\mathcal{R}_{LG}^A)^{-1}\mathcal{R}_{LG}^B\tilde{\mathbf{S}}_B - 2K(\tilde{\mathbf{S}}_A\cdot\tilde{\hat{z}}_A)\tilde{\hat{z}}_A\Big] \\
&+\frac{\alpha_A}{S}\tilde{\mathbf{S}}_A \times \left\{\tilde{\mathbf{S}}_A \times \Big[-\gamma\tilde{\mathbf{B}}_A - J(\mathcal{R}_{LG}^A)^{-1}\mathcal{R}_{LG}^B\tilde{\mathbf{S}}_B - 2K(\tilde{\mathbf{S}}_A\cdot\tilde{\hat{z}}_A)\tilde{\hat{z}}_A\Big]\right\} \qquad \text{(S.7)} \\
(1+\alpha_B^2)\frac{\mathrm{d}\tilde{\mathbf{S}}_B}{\mathrm{d}t} =&\tilde{\mathbf{S}}_B \times \Big[-\gamma\tilde{\mathbf{B}}_B - J(\mathcal{R}_{LG}^B)^{-1}\mathcal{R}_{LG}^A\tilde{\mathbf{S}}_A - 2K(\tilde{\mathbf{S}}_B\cdot\tilde{\hat{z}}_B)\tilde{\hat{z}}_B\Big] \\
&+\frac{\alpha_B}{S}\tilde{\mathbf{S}}_B \times \left\{\tilde{\mathbf{S}}_B \times \Big[-\gamma\tilde{\mathbf{B}}_B - J(\mathcal{R}_{LG}^B)^{-1}\mathcal{R}_{LG}^A\tilde{\mathbf{S}}_A - 2K(\tilde{\mathbf{S}}_B\cdot\tilde{\hat{z}}_B)\tilde{\hat{z}}_B\Big]\right\}, \qquad \text{(S.8)}
\end{aligned}$$

where $\tilde{\mathbf{B}}_i = (\mathcal{R}_{LG}^i)^{-1}\mathbf{B}_0$ and $\tilde{\hat{z}}_i = (\mathcal{R}_{LG}^i)^{-1}\hat{z}$. Plugging the Holstein-Primakoff transformation (S.4) into Eqs. (S.7) and (S.8), truncating beyond the quadratic terms in the Holstein-Primakoff boson operators, and invoking Heinseberg equation of motion, we find the effective non-Hermitian BdG Hamiltonian as

$$\begin{aligned}
H_{nh} =& \frac{1}{1-i\alpha_A}\frac{S}{2}g_1 a^\dagger a^\dagger + \frac{1}{1-i\alpha_A}\frac{S}{2}g_1 aa + \frac{1}{1-i\alpha_B}\frac{S}{2}g_4 b^\dagger b^\dagger + \frac{1}{1-i\alpha_B}\frac{S}{2}g_4 bb \\
&+\frac{1}{2(1-i\alpha_A)}(-f_3+Sg_1-2Sg_2-h_9S)a^\dagger a + \frac{1}{2(1-i\alpha_A)}(-f_3+Sg_1-2Sg_2-h_9S)aa^\dagger \\
&+\frac{1}{2(1-i\alpha_B)}(-f_6+Sg_4-2Sg_5-h_9S)b^\dagger b + \frac{1}{2(1-i\alpha_B)}(-f_6+Sg_4-2Sg_5-h_9S)bb^\dagger \\
&+\frac{1}{\sqrt{(1-i\alpha_A)(1-i\alpha_B)}}\frac{S}{2}(h_1+ih_2+ih_4-h_5)a^\dagger b^\dagger + \frac{1}{\sqrt{(1-i\alpha_A)(1-i\alpha_B)}}\frac{S}{2}(h_1-ih_2-ih_4-h_5)ab \\
&+\frac{1}{\sqrt{(1-i\alpha_A)(1-i\alpha_B)}}\frac{S}{2}(h_1-ih_2+ih_4+h_5)a^\dagger b + \frac{1}{\sqrt{(1-i\alpha_A)(1-i\alpha_B)}}\frac{S}{2}(h_1+ih_2-ih_4+h_5)ab^\dagger, \qquad \text{(S.9)}
\end{aligned}$$

where

$$\begin{aligned}
f_1 =&\gamma B_0(\cos\Theta\cos\phi_A\sin\theta_A - \sin\Theta\cos\theta_A), & f_2 =& -\gamma B_0\cos\Theta\sin\phi_A, \\
f_3 =&\gamma B_0(\cos\Theta\cos\phi_A\cos\theta_A + \sin\Theta\sin\theta_A), & f_4 =&\gamma B_0(\cos\Theta\cos\phi_B\sin\theta_B - \sin\Theta\cos\theta_B), \\
f_5 =& -\gamma B_0\cos\Theta\sin\phi_B, & f_6 =&\gamma B_0(\cos\Theta\cos\phi_B\cos\theta_B + \sin\Theta\sin\theta_B), \\
g_1 =&K\cos^2\theta_A, & g_2 =&K\sin^2\theta_A, \\
g_3 =& -K\cos\theta_A\sin\theta_A, & g_4 =&K\cos^2\theta_B, \\
g_5 =&K\sin^2\theta_B, & g_6 =& -K\cos\theta_B\sin\theta_B, \\
h_1 =&J(\cos\theta_A\cos\theta_B + \cos\phi_{AB}\sin\theta_A\sin\theta_B), & h_2 =&J\sin\theta_A\sin\phi_{AB}, \\
h_3 =&J(\sin\theta_A\cos\theta_B\cos\phi_{AB} - \cos\theta_A\sin\theta_B), & h_4 =& -J\sin\theta_B\sin\phi_{AB}, \\
h_5 =&J\cos\phi_{AB}, & h_6 =& -J\cos\theta_B\sin\phi_{AB}, \\
h_7 =&J(\cos\theta_A\sin\theta_B\cos\phi_{AB} - \sin\theta_A\cos\theta_B), & h_8 =&J\cos\theta_A\sin\phi_{AB}, \\
h_9 =&J(\cos\theta_A\cos\theta_B\cos\phi_{AB} + \sin\theta_A\sin\theta_B).
\end{aligned}$$

and we have redefined the magnon operators as $d_{A(B)} \to a(b)$.
